# Supplementary material for: Combining BART and Principal Stratification to estimate the effect of intermediate variables on primary outcomes with application to estimating the effect of family planning on employment in Nigeria and Senegal
Source: arXiv:2412.16320 source file (2026-03-29)
Supplement: Supplementary file 1 [file Appendices.pdf]

# Appendices to Generalizing causal effect estimates to larger populations while accounting for (uncertainty in) effect modifiers using Bayesian bootstrap with application to estimating the effect of family planning on employment in Nigeria

Lucas Godoy Garraza[1†], Ilene Speizer[2], and Leontine Alkema[1]

[1] Department of Biostatistics and Epidemiology, University of Massachusetts Amherst

[2] Department of Maternal and Child Health, University of North Carolina at Chapel Hill

[†] Contact: lgodoygarraz@umass.edu. This paper was made possible by grants from the Bill & Melinda Gates Foundation and the Children's Investment Fund Foundation. Under the grant conditions, a Creative Commons Attribution 4.0 Generic License has already been assigned to the Author Accepted Manuscript version that might arise from this submission.

## Appendix I Target population(s)

<table>
<tr><th rowspan="2">Variable</th><th rowspan="2">Definition</th><th colspan="3">Population</th></tr>
<tr><th>Urban, same states</th><th>Urban, all states</th><th>Rural and urban, all</th></tr>
<tr><td>Ever use modern contraception</td><td>V302A “ever used anything or tried to delay or avoid getting pregnant” > 0 “no” AND<br>V301 “knowledge of any method” = 3 “knows modern method”</td><td colspan="3">F</td></tr>
<tr><td>Currently using modern contraception</td><td>V313 “current use by method type” = 3 “modern method”</td><td colspan="3">F</td></tr>
<tr><td>Wish to delay or space pregnancy</td><td>V605 “desire for more children” in (“wants after 2+ years”, “wants no more sterilized (respondent or partner)”)</td><td colspan="3">T</td></tr>
<tr><td>Urban</td><td>V025 “Type of place of residence” = “urban”</td><td colspan="2">T</td><td>*</td></tr>
<tr><td>In 5 states</td><td>SSTATE in (Abuja; Edo; Kwara; Kaduna; Oyo)</td><td>T</td><td>*</td><td>*</td></tr>
</table>

*Figure A 1 Definition of target population based on DHS Nigeria dataset NGIR7BFL. “T”: TRUE, “F”: FALSE, “*”: either TRUE or FALSE.*

## Appendix II Additional descriptive characteristics

Table A 1 includes baseline descriptive characteristics for four populations: (1) compliers in the source study, and, based on the 2018 DHS information, (2) all women residing in urban areas in the 5 states represented in the source study, (3) all women residing in urban areas, and (3) all women in Nigeria.

| | | DHS | | |
|---|---|---|---|---|
| Variable | compliers in the source study | all women residing in urban areas in the 5 states represented in the source study | all women residing in urban areas | all women in Nigeria |
| teen_birth (%) | 16.8 (3.2) | 18.0 (1.9) | 16.0 (0.6) | 26.3 (0.6) |
| education | 3.2 (0.1) | 3.1 (0.2) | 3.2 (0.1) | 2.3 (0.0) |
| wealth | 2.8 (0.1) | 2.9 (0.1) | 2.7 (0.1) | 2.0 (0.0) |
| parity | 2.5 (0.3) | 2.8 (0.1) | 2.5 (0.0) | 3.0 (0.0) |
| work_last_year (%) | 56.0 (4.5) | 71.1 (1.8) | 69.9 (0.9) | 68.4 (0.6) |
| work_last_week (%) | 45.2 (4.1) | 70.0 (1.8) | 67.0 (0.9) | 65.0 (0.6) |
| FP_TV (%) | 23.9 (3.8) | 49.7 (3.4) | 30.7 (1.2) | 18.5 (0.8) |
| FP_radio (%) | 48.3 (4.1) | 54.8 (3.3) | 41.6 (1.1) | 31.3 (0.7) |
| knwl_contraception (%) | 91.3 (2.2) | 97.2 (0.4) | 95.5 (0.4) | 92.1 (0.4) |
| paid_cash (%) | 52.3 (4.5) | 65.6 (2.1) | 54.1 (1.0) | 48.0 (0.7) |
| self_employed (%) | 47.2 (4.4) | 55.5 (2.0) | 47.4 (0.8) | 48.2 (0.5) |
| want_no_birth (%) | 54.9 (4.1) | 48.8 (1.8) | 42.3 (0.8) | 43.3 (0.5) |
| had_sex (%) | 68.0 (4.6) | 82.8 (1.5) | 79.6 (0.6) | 83.8 (0.4) |
| att_beat_ok (%) | 31.5 (3.7) | 12.3 (1.7) | 17.6 (1.0) | 28.9 (1.0) |
| never_married (%) | 36.3 (4.9) | 25.6 (1.7) | 32.2 (0.7) | 25.2 (0.6) |
| in_union (%) | 61.2 (4.9) | 70.1 (1.9) | 61.6 (0.8) | 69.5 (0.6) |
| separated (%) | 2.0 (0.8) | 4.3 (0.5) | 6.3 (0.3) | 5.2 (0.2) |

| Variable | compliers in the source study | DHS all women residing in urban areas in the 5 states represented in the source study | all women residing in urban areas | all women in Nigeria |
|---|---|---|---|---|
| age | 26.7 (0.8) | 29.9 (0.2) | 29.3 (0.1) | 29.1 (0.1) |
| age_15_19 (%) | 29.2 (4.5) | 17.4 (0.9) | 19.9 (0.4) | 20.2 (0.3) |
| age_20_24 (%) | 17.1 (3.4) | 16.0 (0.9) | 15.3 (0.3) | 16.4 (0.2) |
| age_25_29 (%) | 17.9 (3.4) | 15.8 (1.0) | 17.0 (0.4) | 17.4 (0.2) |
| age_30_34 (%) | 11.7 (2.6) | 16.6 (0.7) | 15.7 (0.3) | 14.8 (0.2) |
| age_35_39 (%) | 12.6 (2.6) | 14.0 (0.6) | 14.0 (0.3) | 13.1 (0.2) |
| age_40_44 (%) | 6.9 (1.6) | 10.5 (0.6) | 9.3 (0.3) | 9.4 (0.2) |
| age_45_49 (%) | 4.6 (1.3) | 9.6 (0.7) | 8.9 (0.3) | 8.9 (0.2) |
| Muslim (%) | 74.0 (4.5) | 54.3 (5.2) | 45.5 (2.2) | 53.4 (1.5) |
| Christian (%) | 25.3 (4.5) | 45.5 (5.2) | 54.2 (2.2) | 46.0 (1.5) |
| edu_primary (%) | 22.7 (3.2) | 14.4 (1.2) | 13.3 (0.6) | 14.4 (0.4) |
| edu_junioHS (%) | 10.2 (2.6) | 11.6 (1.2) | 10.7 (0.4) | 9.7 (0.3) |
| edu_seniorHS (%) | 38.4 (4.2) | 38.9 (2.8) | 41.8 (0.9) | 30.0 (0.7) |
| edu_higher (%) | 14.5 (3.1) | 18.1 (2.2) | 18.5 (0.9) | 11.0 (0.5) |
| no_edu (%) | 13.3 (2.8) | 17.0 (3.8) | 15.7 (1.1) | 34.9 (1.2) |
| wealth_1 (%) | 22.6 (3.6) | 20.7 (4.0) | 24.2 (1.5) | 52.9 (1.5) |
| wealth_2 (%) | 26.7 (3.5) | 22.0 (2.3) | 23.7 (1.0) | 17.7 (0.6) |
| wealth_3 (%) | 16.0 (2.9) | 21.7 (2.4) | 19.2 (0.8) | 11.6 (0.5) |
| wealth_4 (%) | 20.3 (3.3) | 19.6 (2.0) | 19.5 (0.9) | 10.8 (0.5) |
| wealth_5 (%) | 14.4 (3.3) | 16.0 (2.7) | 13.5 (1.1) | 7.0 (0.6) |
| parity_0 (%) | 39.4 (5.0) | 28.4 (1.4) | 33.8 (0.6) | 28.4 (0.5) |
| parity_1 (%) | 9.0 (2.5) | 10.7 (0.8) | 11.5 (0.4) | 11.3 (0.2) |
| parity_2 (%) | 9.8 (2.3) | 14.5 (1.0) | 12.1 (0.4) | 11.8 (0.2) |
| parity_3 (%) | 11.1 (2.4) | 12.3 (0.8) | 11.3 (0.3) | 10.7 (0.2) |
| parity_4 (%) | 10.5 (2.2) | 10.4 (0.8) | 9.3 (0.3) | 9.4 (0.2) |

| Variable | compliers in the source study | DHS: all women residing in urban areas in the 5 states represented in the source study | all women residing in urban areas | all women in Nigeria |
|---|---|---|---|---|
| parity_5 (%) | 5.5 (1.6) | 7.8 (0.6) | 7.7 (0.4) | 8.2 (0.2) |
| parity_6 (%) | 4.5 (1.4) | 6.1 (0.6) | 5.3 (0.3) | 6.4 (0.2) |
| parity_7 (%) | 10.2 (2.4) | 9.7 (1.5) | 9.0 (0.5) | 13.8 (0.4) |

*Table A 1 Descriptive characteristics for four populations: (1) compliers in the source study, and, based on the 2018 DHS information, (2) all women residing in urban areas in the 5 states represented in the source study, (3) all women residing in urban areas, and (4) all women in Nigeria.*

## Appendix III Additional simulation results

| | Bias | Coverage 95 %CIs | SD | RMSE |
|---|---|---|---|---|
| Naïve (i.e., assuming SRS) | .095 | .657 | .068 | .133 |
| Standard frequentist | -.001 | .951 | .093 | .093 |
| BB | -.001 | .97 | .104 | .093 |

*Table A 2 Performance of naïve (assuming SRS), standard design-based frequentist, and BB approaches for estimating the mean age in a population that is given by the DHS sample with half the PSUs selected randomly. Estimates are based on 1,000 replicated data sets using a stratified two-stage cluster sample with replacement from the true population.*

| | Bias | Coverage 95 %CIs | SD | RMSE |
|---|---|---|---|---|
| Naïve (i.e., assuming SRS) | .105 | .647 | .075 | .149 |
| Standard frequentist | .002 | .942 | .103 | .107 |
| BB | .002 | .963 | .116 | .107 |

*Table A 3 Performance of naïve (assuming SRS), standard design-based frequentist, and BB approaches for estimating the mean age in a population that is given by the DHS sample with PSUs from urban strata only. Estimates are based on 1,000 replicated data sets using a stratified two-stage cluster sample with replacement from the true population.*

| | Est | SD | 95%CI | |
|---|---|---|---|---|
| | | | LW | UP |
| Naïve (assuming SRS) | .112 | .003 | .107 | .118 |
| Standard frequentist | .118 | .004 | .109 | .126 |
| BB | .118 | .005 | .108 | .127 |

*Table A 4 Estimated proportion of women 15 to 19 years old using naïve (assuming SRS), standard design-based frequentist, and BB approaches based on the actual DHS sample.*
